# Supplementary material for: Extending ALCQIO with reachability
Source: arXiv:1402.6804 source file (2014-07-09)
Supplement: Supplementary file 1 [file appendix-backwards.tex]

\section{Backwards propagation}
\label{se:backwards-app}\label{app:backward}

Here we give the exact formulation of the backwards propagation lemma
and prove it. 

It is convenient to consider a program $\overline{S}$, which behaves like $S$, except that it does not abort. 
$\overline{S}$ uses a fresh variable $abo$ to indicate whether $S$ aborts. 
 The command $abo := \false$ is added at the beginning of the code.
 Every command $C$ of the form $var_1 := var_2.f$, $var_2.f := var_1$ or $dispose(var_2)$ is replaced with $\overline{C} = if\,\, var_2\,\, =\,\, \nil\,\, then\,\, abo := \true\,\, else\,\, C\,\, fi$.
 For $if$, $assume$ and assignments of the form $var_1.f_1 := var_2.f_2$ commands the case is similar, except that there may be two evaluations
of the form $var_i.f_j$, which need to be reflected in the condition in $\overline{C}$.
By the construction of $\overline{S}$, $\overline{S}$ has the following properties:
\begin{enumerate}
 \item The run of $\mm_1$ on $\overline{S}$ does not abort for any $\mm_1$. 
 \item $abo$ has the value $\true$ at the end of the run of $\overline{S}$ on $\mm_1$
if and only if $S$ aborts on $\mm_1$.
 \item If $\left\langle S,\mm_1\right\rangle\leadsto \mm_2$, then $\left\langle \overline{S},\mm_1\right\rangle\leadsto \mm_2$. 
\end{enumerate}

We need a further extension of our structures, which uses a refined $\leadsto$ relation. 
The refined $\leadsto$ relation will get rid of some non-determinism in the semantics of the programming language. 

Given a finite set $Y$ of labels and a tuple $\bar{d}_Y=(d_y: y\in Y)$ of elements of $M$,
we denote by $\left\langle \mm_1, (\bar{R}^{ext})^{\mm_1}, \bar{d}_Y \right\rangle$
the structure obtained from $\left\langle \mm_1, (\bar{R}^{ext})^{\mm_1}\right\rangle$ by adding the constants $d_y$ for each $y\in Y$.
The vocabulary $\tau_{Y}^{ext}$ of $\left\langle \mm_1, (\bar{R}^{ext})^{\mm_1}, \bar{d}_Y \right\rangle$ extends
$\tau^{ext}$ by constant symbols $\{o_y: y\in Y\}$. 

Given a loopless program $S'$, we assign unique labels $y$ to the commands of $S'$.
For any loopless program $S'$, we denote by $Y_{S'}$ the set of labels of commands in $S'$.
The $\leadsto_{{\bar{d}_{Y_S'}}}$ relation is obtained from the $\leadsto$ relation as follows:\\
$\left\langle S',\mm_1\right\rangle\leadsto_{\bar{d}_{Y_{S'}}}  \mm_2$ iff $\left\langle S',\mm_1\right\rangle\leadsto \mm_2$, except in the three following cases
for $S'$:
\begin{itemize}
 \item[--] $y: var_1 := var_2.f$: $\left\langle S',\mm_1\right\rangle\leadsto_{d_y}  \mm_2$ iff 
 $\left\langle S',\mm_1\right\rangle\leadsto  \mm_2$ and  $f^{\mm_1}(o_{var_2}^{\mm_1})=d_y$. 
           Else, $\left\langle S',\mm_1\right\rangle\leadsto_{d_y} \abo$. 
 \item[--] $y: var:=new$: $\left\langle S',\mm_1\right\rangle\leadsto_{d_y}  \mm_2$ iff 
 $\left\langle S',\mm_1\right\rangle\leadsto  \mm_2$ and  $o_{var}^{\mm_2}=d_y$. 
           Otherwise, $\left\langle S',\mm_1\right\rangle\leadsto_{d_y} \abo$. 
 \item[--] $S'_1; S'_2$: If $\left\langle S'_1,\mm_1\right\rangle\leadsto_{\bar{d}_{Y_{S'_1}}}  \mm'$ and
$\left\langle S'_2,\mm'\right\rangle\leadsto_{\bar{d}_{Y_{S'_2}}}  \mm_2$, 
then $\left\langle S'_1;S'_2,\mm_1\right\rangle\leadsto_{\bar{d}_{Y_{S'_1}}\cup\bar{d}_{Y_{S'_2}}}  \mm_2$. 
\end{itemize}
The main observation is:
\begin{lemma}
For any two memory structures $\mm_1$ and $\mm_2$, 
$\left\langle S',\mm_1\right\rangle\leadsto \mm_2$ iff there exists a tuple $\bar{d}_{Y_S'}$ such that
$\left\langle S',\mm_1\right\rangle\leadsto_{\bar{d}_{Y_S'}}  \mm_2$ .
\end{lemma}

We are now ready to state Lemma \ref{lem:backwards--} precisely:
\begin{lemma}\label{lem:backwards-app} \label{se:backwards-ghost-app}
Let $S$ be a loopless program, $Y_{\overline{S}}$ be the set of labels of commands in $\overline{S}$,
$\mm_1$ and $\mm_2$ be  memory structures, $\bar{d}_{Y_{\overline{S}}}$ be a tuple of $M$ elements
labeled with the labels in $Y_{\overline{S}}$, $d_{abo}\in M$, and
 $\varphi$ be an $\L$-formula over $\tau$.
\begin{enumerate}
 \item If $\left\langle S, \mm_1\right\rangle \leadsto_{\bar{d}_{Y_{\overline{S}}}} \mm_2$, 
 then:\\
 $\mm_2\models \varphi$ iff
$\left\langle \mm_1, (\bar{R}^{ext})^{\mm_1}, \bar{d}_{Y_{\overline{S}}}, d_{abo} \right\rangle \models \Theta_{S}(\varphi)$.
\item If $\left\langle S, \mm_1\right\rangle\leadsto_{\bar{d}_{Y_{\overline{S}}}}  \abo$, then
  for every tuple $\bar{d}_{Y_{\overline{S}}}$ of $M$ elements, 
$\left\langle \mm_1, (\bar{R}^{ext})^{\mm_1},
\bar{d}_{Y_{\overline{S}}},d_{abo} \right\rangle \not\models \Theta_{S}(\varphi)$.
\end{enumerate}
The vocabulary of the structure $\left\langle \mm_1, (\bar{R}^{ext})^{\mm_1}, \bar{d}_{Y_{\overline{S}}}, d_{abo} \right\rangle$ is 
$\tau^{ext}_{Y_{\overline{S}}} \cup\{o_{abo}\}$. 

The definition of $\Theta_S$ is:
\begin{definition}$\Theta_{S}(\varphi)=\Phi_{\overline{S}}(\varphi\land (o_{abo} \equiv o_\false)))$,
$\Phi$ is obtained from $\Psi$ by
substituting every  symbol $R\in\tau^{rem}$ in $\varphi$ by $R^{ext}$, and
$\Psi$ is defined as:
\[\begin{array}{lll}
\Psi_{skip}(\varphi) &=&\varphi\\
\Psi_{var_{1}:=e}(\varphi)&=&\varphi[{o_{var_{1}} /  o_{e}}],\, e=var_{2}\mbox{ or }e=\nil\\
\Psi_{y: var_{1}:=var_{2}.f}(\varphi)&=&\varphi[o_{var_{1}} / o_y] \land (\exists f^{-}.o_{var_{2}}\equiv o_y)\\
\Psi_{var_{1}.f:=e}(\varphi)&=&\varphi[f / f\backslash(o_{var_{1}}\times\top)\cup(o_{var_{1}},o_{e})],\, \\
&&\mbox{where }e=var_{2}\mbox{ or }e=\nil\\
\Psi_{if\,\, b\,\, then\,\,  S_{1}\,\, else\,\, S_{2}\,\, fi}
%\substack
(\varphi)&=&\varepsilon_{b}\land\Psi_{S_{1}}(\varphi)\lor\neg\varepsilon_{b}\land\Psi_{S_{2}}(\varphi)\\
\Psi_{y:var:=new}(\varphi)&=&\varphi[o_{var} /  o_{y}][Alloc / Alloc\sqcup o_{y}] \\
&&\land o_y\sqsubseteq \neg Alloc\\
\Psi_{dispose(var)}(\varphi)&=&\Psi_{S_{disp}}(\varphi[Alloc / Alloc\sqcap\neg o_{var}]),\\
&&\mbox{where }S_{disp}=var.f_{k_1} := \nil; \\ 
 && \cdots;  var.f_{k_w} := \nil\\
\Psi_{S_{1};S_{2}}(\varphi)&=&\Psi_{S_{1}}(\Psi_{S_{2}}(\varphi)) \
\end{array}
\]
The notation $\varphi[A / B]$ should be interpreted as
the syntactic replacement of any occurrence of $A$ with $B$.
We write e.g. $y: var:= new$ to indicate that the command $var := new$ is labeled with $y$.
$\varepsilon_{b}$ is defined inductively:
for
$e_{1}=e_{2}$ we set $\varepsilon_{b}=(A_{e_{1}}\equiv A_{e_{2}})$,
with $A_{var}=o_{var}$ and $A_{var.f}=\exists f^{-}.o_{var}$; $\varepsilon$
extends naturally to the Boolean connectives.
In the definition of $\Psi_{dispose(var)}$, $f_{k_1},\ldots,f_{k_w}$ are the members of $\tauField$ which
occur in $\varphi$. W.l.o.g. we assume that $S$ does not contain commands of the form $if\,\,b\,\,then\,\,S_1\,\, fi$
or $var_1.f_1 := var_2.f_2$, since they can be expressed using the other commands.
\end{definition}
\end{lemma}

To prove Lemma \ref{lem:backwards-app} we need the following lemma:

\begin{lemma}\label{lem:backwards2-app}
Let $S$ be a loopless program without $assume$ commands, $Y_S$ be the set of labels of commands in $S$,
$Y$ be a set of labels disjoint from $Y_S$,
$\mm_1$ and $\mm_2$ be memory structures with universe $M$
and $\bar{d}_{Y_S}$ a tuple of $M$ elements
such that 
$\left\langle S, \mm_1\right\rangle\leadsto_{\bar{d}_{Y_S}} \mm_2$.
% and $(\nn_1)_{\gho} = (\nn_2)_{\gho}$,
Let $\bar{d}_Y$ be a tuple of $M$ elements and
 $\varphi$ be an $\L$-formula over $\tau\cup\{o_{y}: y\in Y\}$.
$\left\langle \mm_2, \bar{d}_Y \right\rangle\models \varphi$ iff
$\left\langle \mm_1, (\bar{R}^{ext})^{\mm_1}, \bar{d}_Y, \bar{d}_{Y_S} \right\rangle \models \Phi_S(\varphi)$.
\end{lemma}

\begin{proof}
We prove the lemma by induction.
\begin{itemize}
\item $S=skip$: $Y_S = \emptyset$, and we have $\left\langle \mm_2, \bar{d}_Y \right\rangle\models \varphi$
      iff $\left\langle \mm_1, \bar{R}^{ext}, \bar{d}_Y \right\rangle\models \Phi_S(\varphi)$, as required.
\item $S = if\,b\,then\,S_1\,else\,S_2\, fi$: depending on whether $\varepsilon_b$ is true or false, $\Phi_{S_1}(\varphi)$ or $\Phi_{S_2}(\varphi)$
      should be used.
\item $var_1 := e$, where $e$ is a variable $var_2$ or $\nil$: every reference to $var_1$ in $\varphi$ is replaced
      by a reference to $var_2$ or $\nil$, respectively.
\item $var_1 := var_2.f$: every reference to $var_1$ in $\varphi$ is replaced with a reference to $o_y$, whose interpretation is $d_y$,
      in accordance with $\leadsto_{\bar{d}_{Y_S}}$, which requires that $d_y$ be the result of applying $f$ on $var_2$.
\item $var_1.f := e$, where $e$ is a variable $var_2$ or $\nil$: the function symbol $f$ is updated by
      removing the current value of $f$ on $var_1$ by subtracting $(o_{var_{1}}\times\top)^{\mm_1}$ from $f^{\mm_1}$
      and setting the new value explicitly
      by adding the pair $(o_{var_1}^{\mm_1},o_{e}^{\mm_1})$ to $f^{\mm_1}$.
\item $S= var := new$ with label $y$: $Y_S = \{y\}$ and $\bar{d}_{Y_S}=(d_y)$. By the definition of $\leadsto_{\bar{d}_{Y_S}}$
      for $new$ commands, $\{d_y\} = Alloc^{\mm_2}\backslash Alloc^{\mm_1}$.
      $\Phi_S(\varphi)$ adds $o_y$ to $Alloc$ and replaces
      every reference to $var$ by a reference to $o_y$.

\item $S = dispose(var)$: $\Phi_S(\varphi)$ removes $var$ from $Alloc$, and using an application of $\Phi$
      to the program $var.f_{k_1} := \nil; \cdots; var.f_{k_w} := \nil$, sets all of the fields
      in $\varphi$ to $\nil$.
\item $S=S_1;S_2$: $\Phi_S(\varphi) = \Phi_{S_1}(\Phi_{S_2}(\varphi))$.
      Let $\mm_3$ be an memory structure such that
      $\left\langle S_1,  \mm_1 \right\rangle\leadsto_{\bar{d}_{Y_{S_1}}} \mm_3$ 
      and $\left\langle S_2,  \mm_3 \right\rangle\leadsto_{\bar{d}_{Y_{S_2}}} \mm_2$.
      We have ${\bar{d}_{Y_{S}}} ={\bar{d}_{Y_{S_1}}}\cup {\bar{d}_{Y_{S_2}}}$.  
      %and
      %$(\nn_1)_{\go} = (\nn_3)_{\gho}$. 

      Consider first $\Phi_{S_2}(\varphi)$. By the induction hypothesis, 
      $\left\langle \mm_2, \bar{d}_Y \right\rangle\models \varphi$ iff
      $\left\langle \mm_3,  \bar{R}^{\mm_2}, \bar{d}_Y, \bar{d}_{Y_{S_2}} \right\rangle \models \Phi_{S_2}(\varphi)$. 

      Let $\mm_4$ be obtained from $\mm_3$ be replacing every relation $R^{\mm_3}$ with $R^{\mm_2}$ for $R\in \tau^{rem}$.
      We have 
      $\Psi_{S_2}(\varphi) \models \left\langle \mm_4,\bar{d}_Y, \bar{d}_{Y_{S_2}} \right\rangle$ 
      iff $ \Phi_{S_2}(\varphi) \models \left\langle \mm_3,  \bar{R}^{\mm_2}, \bar{d}_Y, \bar{d}_{Y_{S_2}} \right\rangle$.

      Since we have $\left\langle S_2,  \mm_4 \right\rangle\leadsto_{\bar{d}_{Y_{S_2}}} \mm_2$, 
      we can apply the induction hypothesis once again, this time on $\Psi_{S_2}$.
      We get that 
      $\left\langle \mm_4, \bar{d}_Y, \bar{d}_{Y_{S_2}} \right\rangle\models \varphi$ iff
      $\left\langle \mm_1,  \bar{d}_Y, \bar{d}_{Y_{S_2}}, \bar{d}_{Y_{S_1}} \right\rangle \models \Phi_{S_1}(\Phi_{S_2}(\varphi))$.
      Hence, 
      $\left\langle \mm_2, \bar{d}_Y \right\rangle\models \varphi$ iff
      $\left\langle \mm_1, \bar{R}^{\mm_2}, \bar{d}_Y, \bar{d}_{Y_{S}} \right\rangle \models \Phi_{S_1}(\Phi_{S_2}(\varphi))$.

\end{itemize}

\end{proof}

\begin{proof}[Proof of Lemma \ref{lem:backwards-app}]

Using Lemma \ref{lem:backwards2-app} with $Y=\emptyset$,
if $\left\langle S, \mm_1\right\rangle\leadsto_{\bar{d}_{Y_S}} \abo$, then
for every tuple of relations $\bar{U}$ interpreting $\bar{R}^{ext}$ we have
$\left\langle \mm_1, \bar{U}, \bar{d}_{Y_S}, d_{abo} \right\rangle \not\models \Phi_{\overline{S}}(\varphi\land (o_{abo} \equiv o_\false))$,
because $abo$ is set to true during the run of $\overline{S}$. 
If $\left\langle S, \mm_1\right\rangle\leadsto_{\bar{d}_{Y_S}} \mm_2$,
% and 
%$(\nn_1)_{\gho} = (\nn_2)_{\gho}$, then there exists $\bar{d}_{Y_S}$ and $d_{abo}$ such that
$\mm_2 \models \varphi$  iff
$\left\langle \mm_1, \bar{d}_{Y_S}, d_{abo} \right\rangle \models \Phi_{\overline{S}}(\varphi\land (o_{abo} \equiv o_\false))$.

Note that $d_{abo}$ is the value of $abo$ at the beginning of the run of $\overline{S}$.
Since the first command of $\overline{S}$ assigns $abo$ a new value, $d_{abo}$ plays no role (it appears because, technically, $abo$ still needs a value at the beginning of the run).

Also note that in Lemma \ref{lem:backwards--}, $\bar{d}_{Y_{\overline{S}}}$ strictly extends $\bar{d}_{Y_S}$, since
$\overline{S}$ extends $S$. However, the semantics of all of the new commands in $\overline{S}$ does not actually
depend on the relevant $d_y$ (since none of them of $new$ commands or assignments of the form $var_1.var_2.f$). 
Hence, any extension of  $\bar{d}_{Y_S}$ into $\bar{d}_{Y_{\overline{S}}}$ will do. 
\end{proof}

\begin{remark}
Revisiting the example in Section \ref{se:backwards-example} with the detailed version of Lemma \ref{lem:backwards-app} in mind,
we now see that $\Theta$ is actually the backwards propagation of programs of the form $\overline{S}$. 
The backward propagation of $\overline{\lambda(\ell_l.\ell_l)}$ is similar to that presented in Section
\ref{se:backwards-example}, with 
$\Theta_{\overline{\lambda(\ell_l.\ell_l)}}(\varphi_{p-as-\ell_l}) = \Phi_{\overline{\lambda(l.l)}}(\varphi_{p-as-\ell_l}\land
(o_{abo} \equiv o_\false))$. 

\end{remark}
